# Supplementary material for: Memory Efficient Matting with Adaptive Token Routing
Source: arXiv:2412.10702 source file (2024-12-17)
Supplement: Supplementary file 1 [file ab_components.tex]

\begin{table}
\centering
\setlength{\tabcolsep}{3.2pt}
\begin{tabular}{ccc|cccc}
\toprule
 LG & DWC & ECA & SAD $\downarrow$ & MSE $\downarrow$ & Mem$_{/\text{GB}}$ & Latency$_{/\text{ms}}$  \\ \midrule
\rowcolor[HTML]{d7dbdd}
  \ding{51} & \ding{51} & \ding{51} & \textbf{21.90} & \textbf{3.37}  & \textbf{0.71}   & \textbf{83.43}   \\
  \midrule

  \ding{55} & \ding{51} & \ding{51} & 22.15 & 3.42 & 1.06 & 86.50 \\
  \ding{51}   & \ding{55} & \ding{51} & 22.23 & 3.49 & 1.06 & 91.09\\
  \ding{51}  & \ding{51} & \ding{55} & 22.09 & 3.53 &1.07 & 90.87 \\

\bottomrule

\end{tabular}
\caption{Effect of different components in the router and LTRM. LG denotes local-global strategy in the router. DWC and ECA represent depth-wise convolution and efficient channel attention in the LTRM, respectively. The default setting is marked in gray.
}
\label{tab:ab_components}
\end{table}
